# Supplementary material for: FMM-Head: Enhancing Autoencoder-based ECG anomaly detection with prior knowledge
Source: arXiv:2310.05848 source file (2023-10-06)
Supplement: Supplementary file 1 [file Appendix.tex]

\newpage

\section{Appendix}
\label{sec:appendix}
